# Supplementary material for: Whispers of Doubt Amidst Echoes of Triumph in NLP Robustness
Source: arXiv:2311.09694 source file (2024-04-03)
Supplement: Supplementary file 1 [file appendix_comment_splits.tex]

\begin{figure*}[t]
  \centering
    \centering
    \begin{minipage}[t]{0.72\textwidth}
        \centering
        \begin{subfigure}{\textwidth}
            \includegraphics[width=\linewidth]{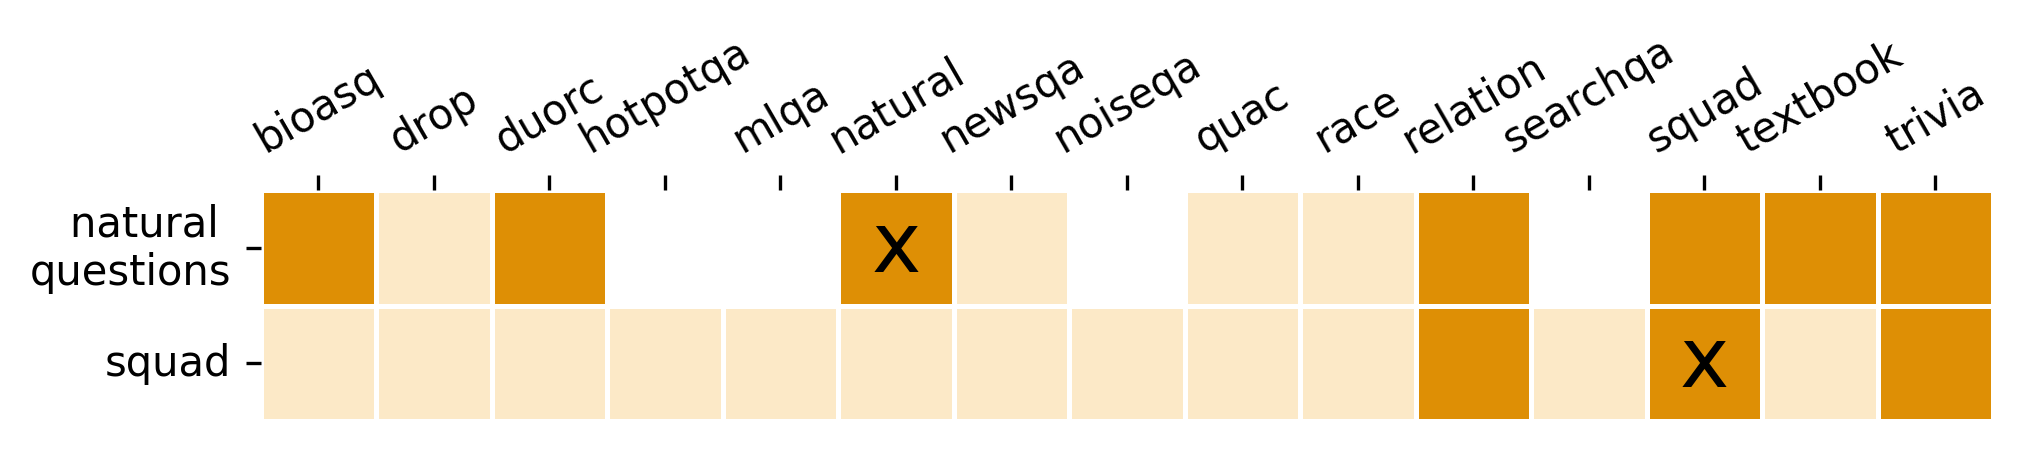}
            \caption{Reading Comprehension}
            \label{fig:mistral_qa_heatmap}
        \end{subfigure}
    \end{minipage}
    \begin{minipage}[t]{0.15\textwidth}
        \centering
        \begin{subfigure}{\textwidth}
            \includegraphics[width=\linewidth]{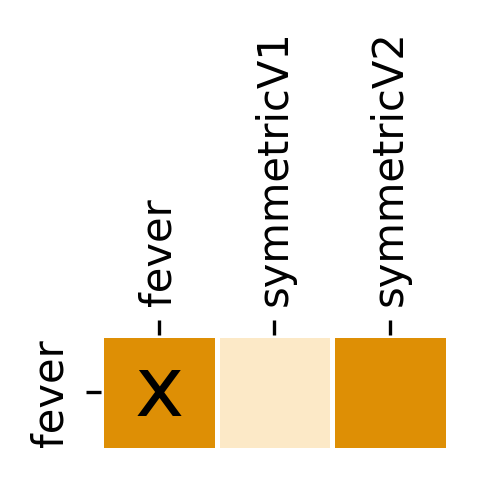}
            \caption{Claim Verif.}
        \end{subfigure}
    \end{minipage}
    \begin{minipage}[t]{0.11\textwidth}
        \centering
        \begin{subfigure}{\textwidth}
            \includegraphics[width=\linewidth]{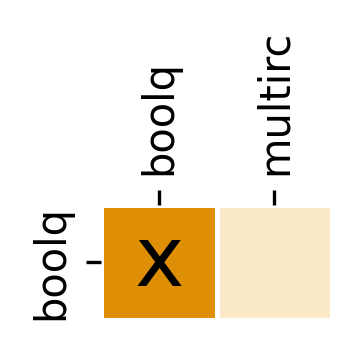}
            \caption{QA}
        \end{subfigure}
    \end{minipage}
    \begin{minipage}[b]{0.47\textwidth}
        \centering
        \begin{subfigure}{\textwidth}
            \includegraphics[width=\linewidth]{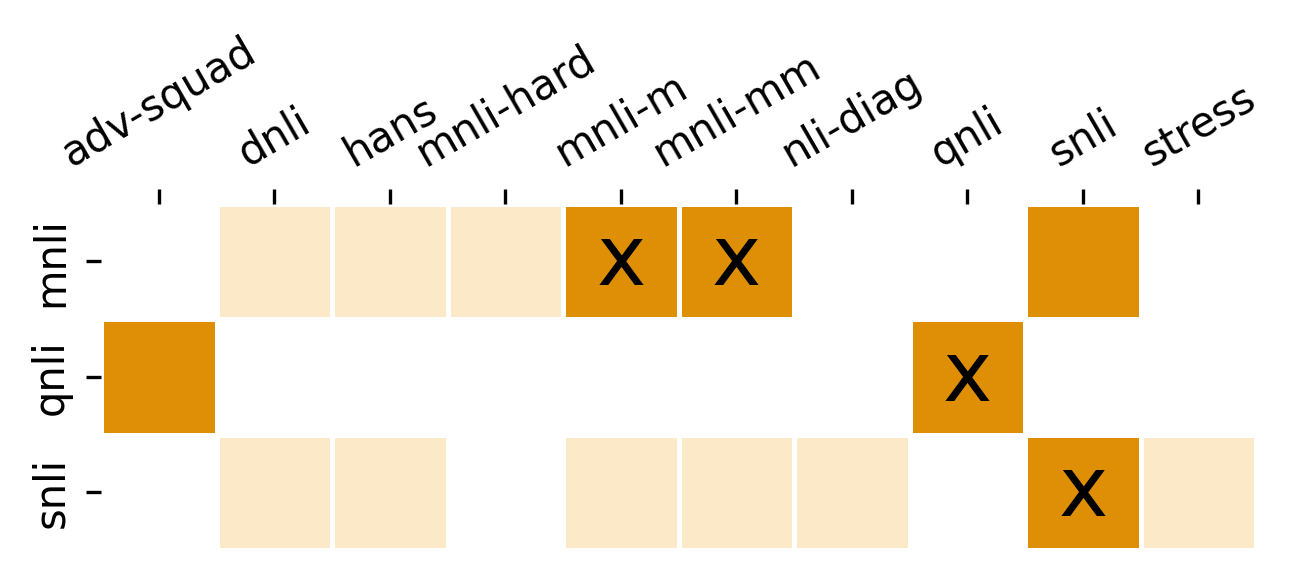}
            \caption{Natural Language Inference}
        \end{subfigure}
    \end{minipage}
    \begin{minipage}[b]{0.28\textwidth}
        \centering
        \begin{subfigure}{\textwidth}
            \includegraphics[width=\linewidth]{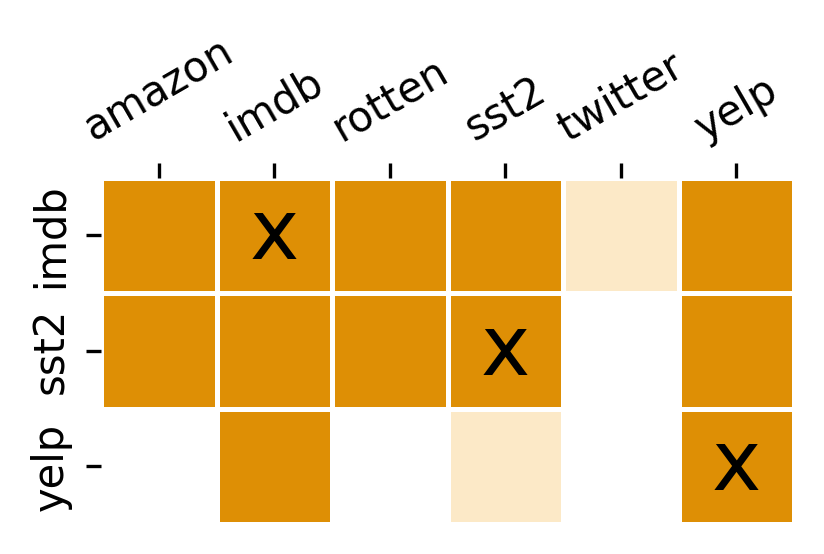}
            \caption{Sentiment Classification}
        \end{subfigure}
    \end{minipage}
    \begin{minipage}[b]{0.23\textwidth}
        \centering
        \begin{subfigure}{\textwidth}
            \includegraphics[width=\linewidth]{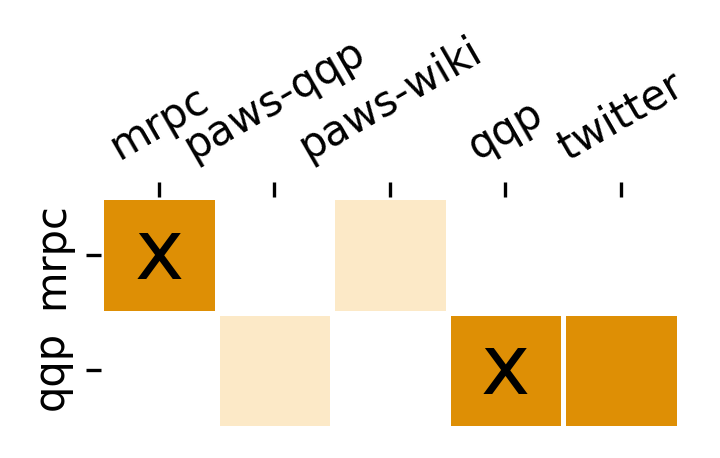}
            \caption{Paraphrase Identification}
            \label{fig:mistral_paraphrase_heatmap}
        \end{subfigure}
    \end{minipage}
  \begin{subfigure}{\textwidth}
    \centering
    \includegraphics[width=\textwidth]{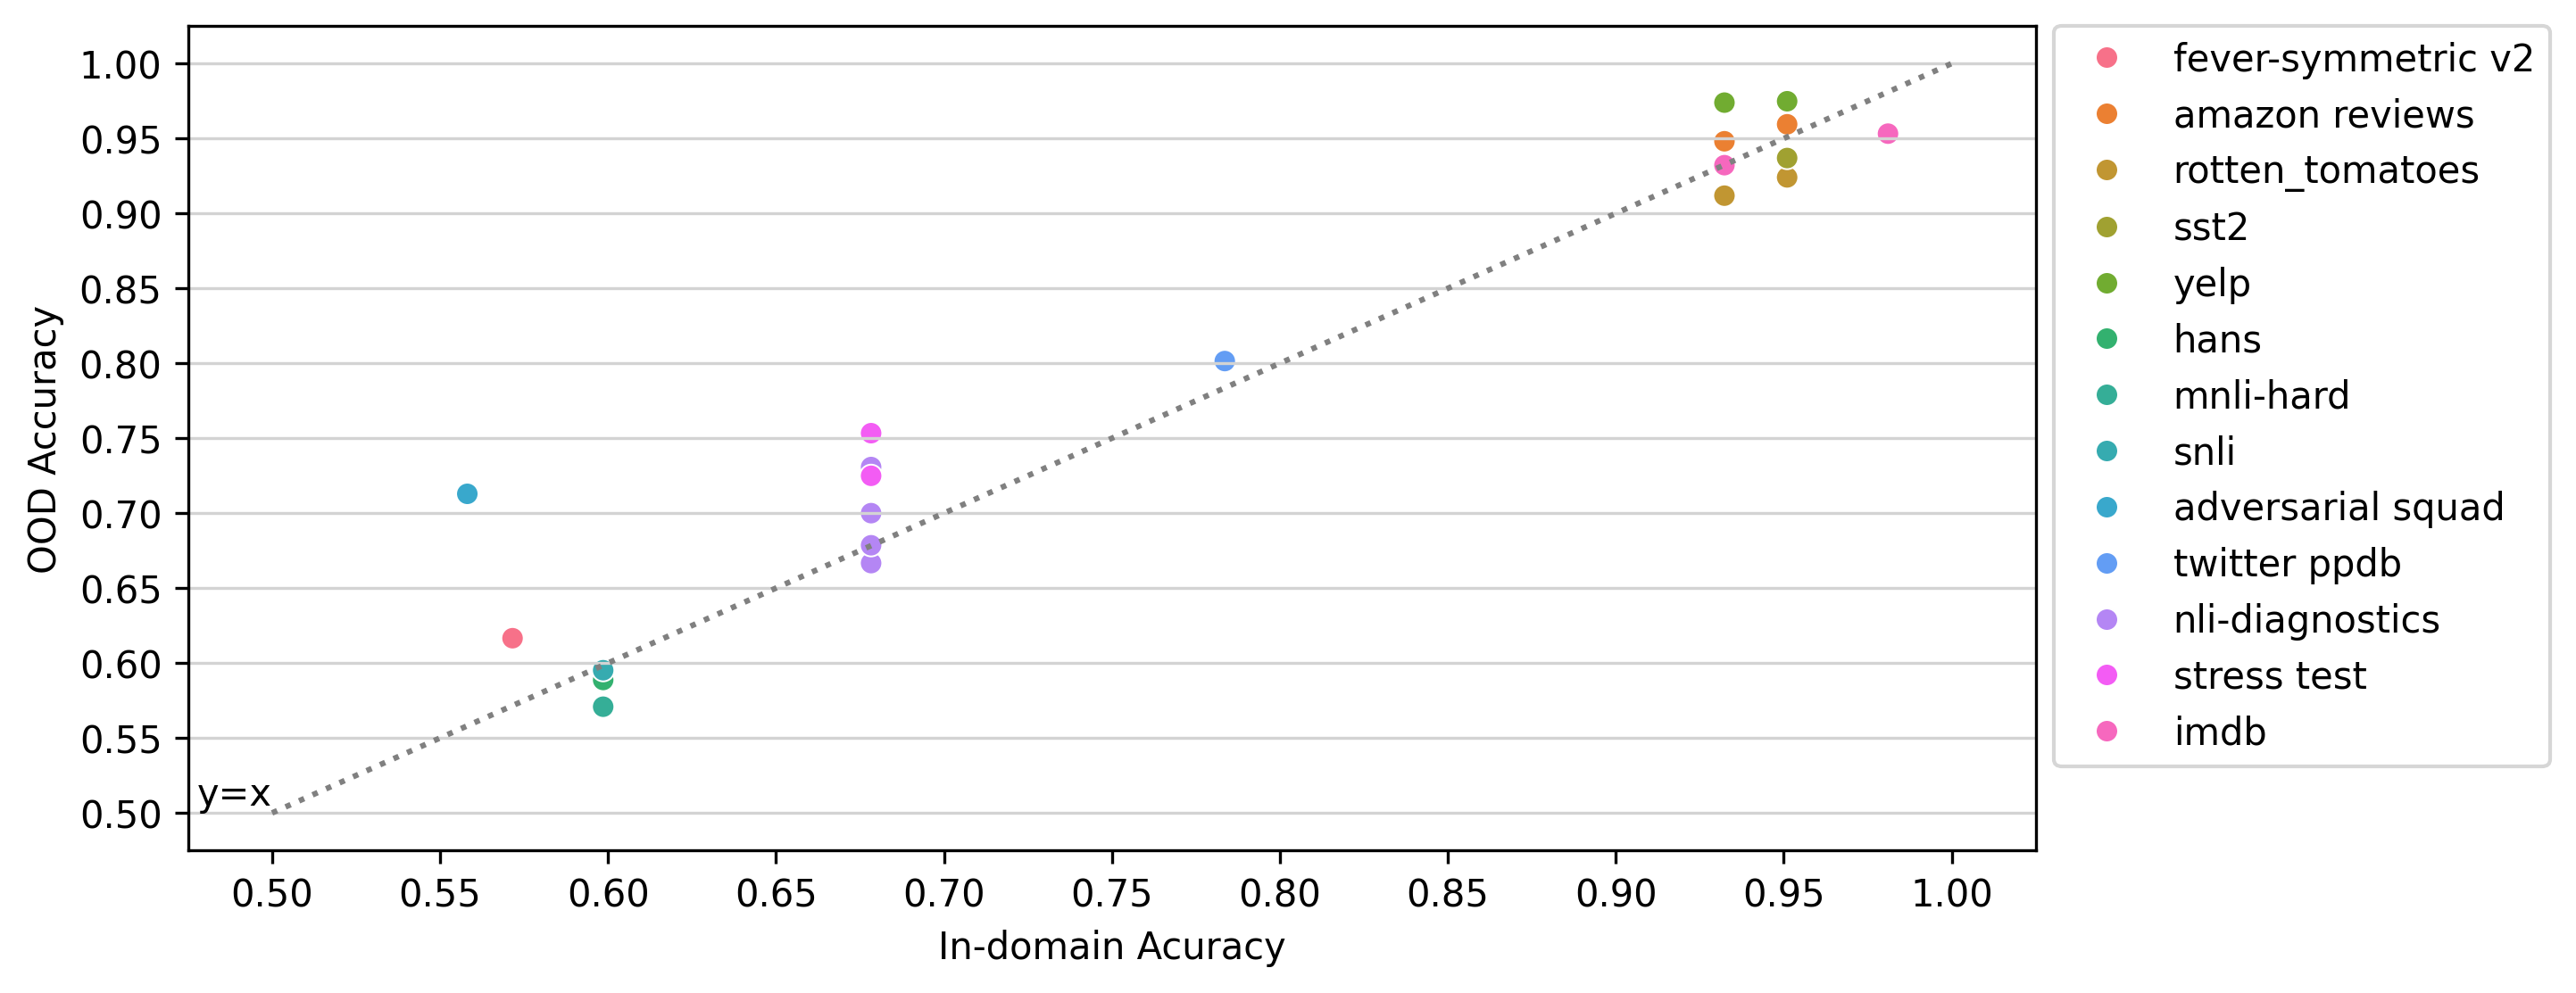}
    \caption{Each point is associated with a train-test split for which Mistral-7B gets OOD accuracy that is at most 3\% worse, if at all, than in-domain accuracy.}
    \label{fig:ood_icl_unproblematic_splits}
  \end{subfigure}
  \begin{subfigure}{\textwidth}
    \centering
    \includegraphics[width=\textwidth]{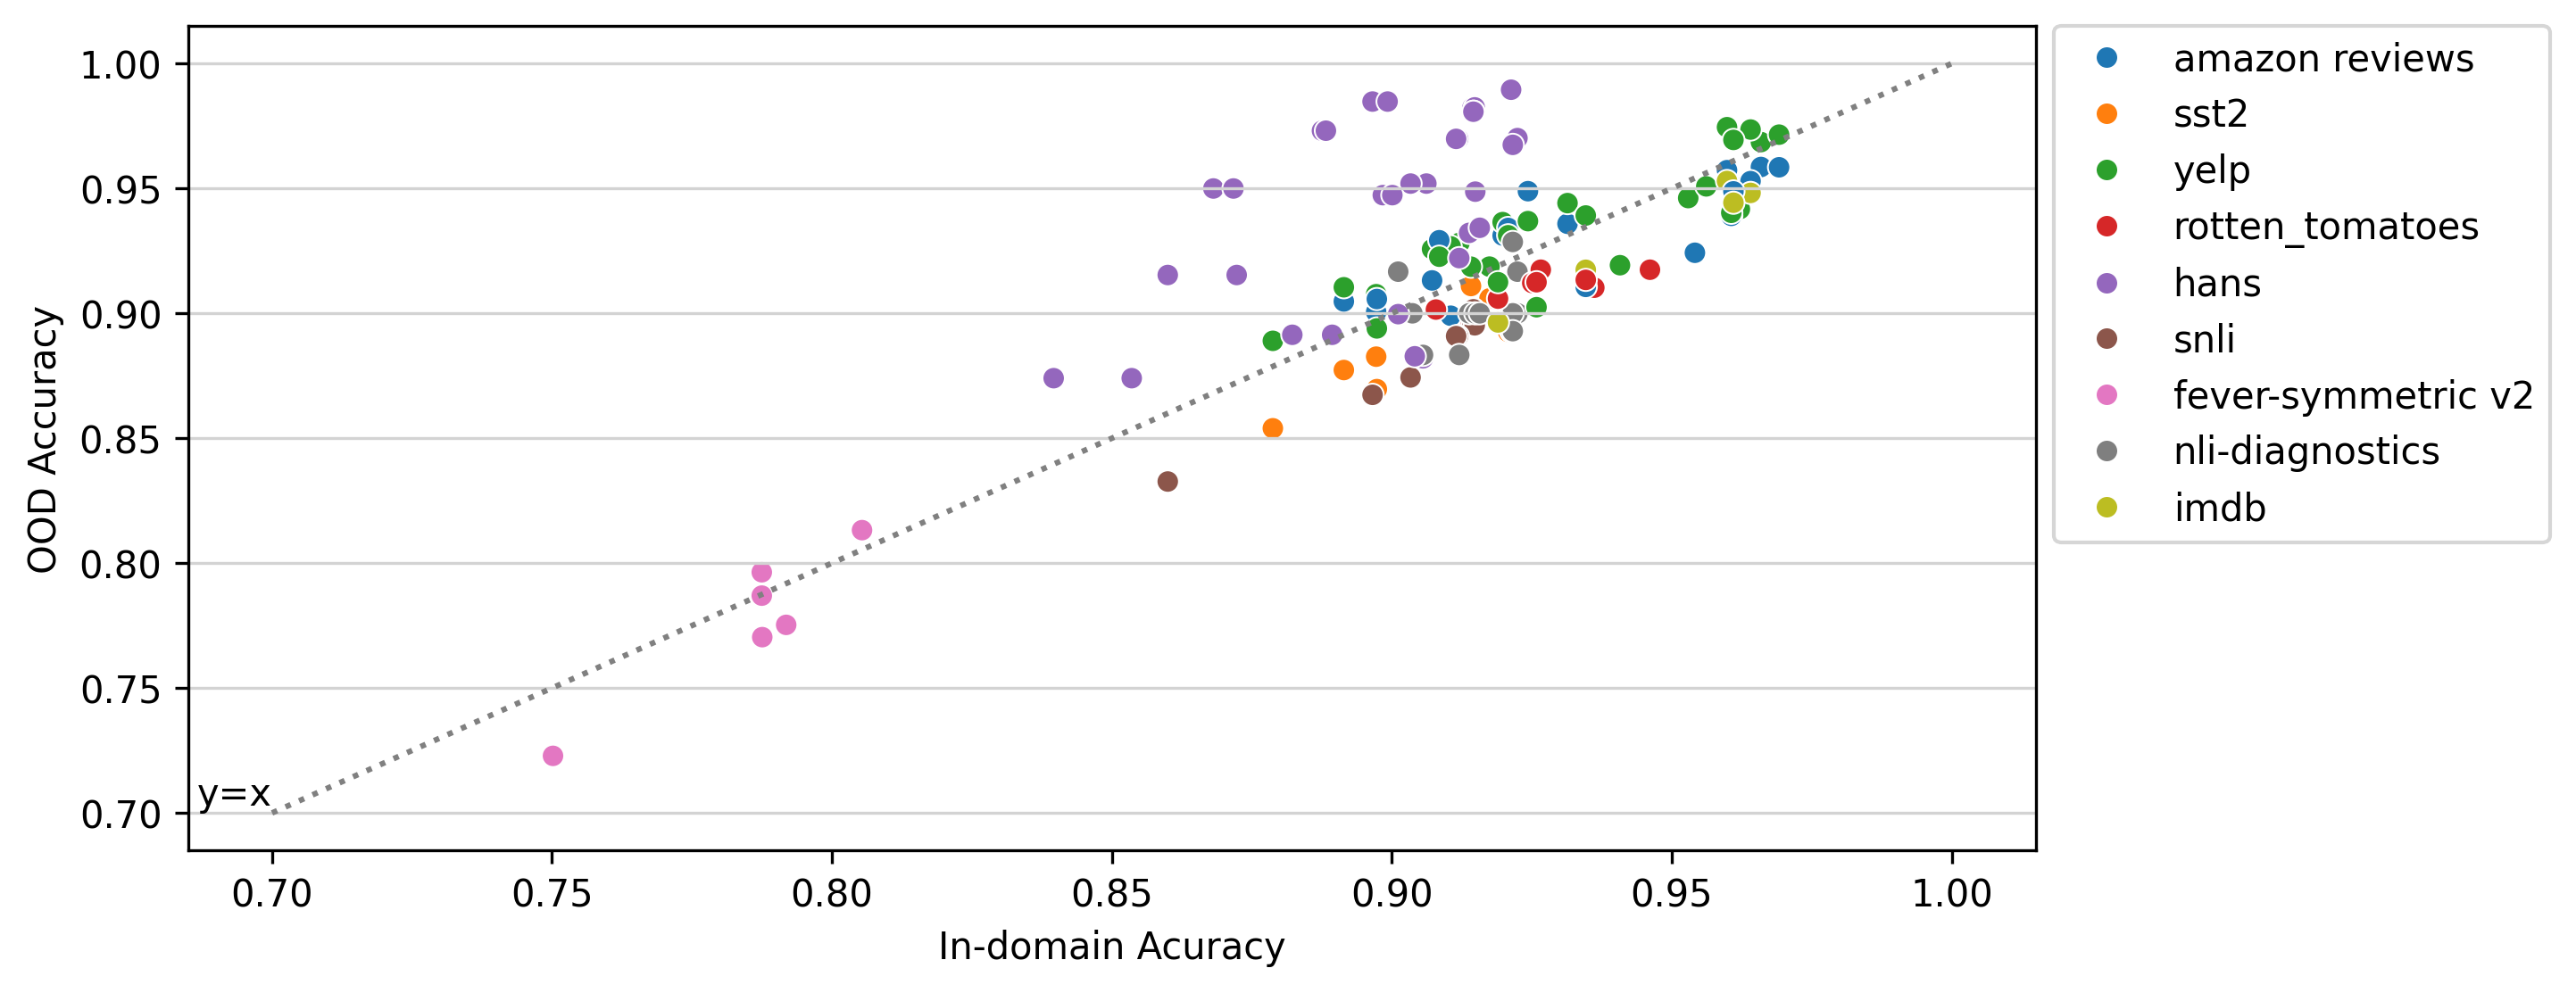}
    \caption{Each point is associated with a train-test split and a finetuned model. In this data split, the model gets  OOD accuracy that is at most 3\% worse, if at all, than in-domain accuracy.}
    \label{fig:ood_finetuned_unproblematic_splits}
  \end{subfigure}
  \caption{Subfigures \ref{fig:mistral_qa_heatmap}--\ref{fig:mistral_paraphrase_heatmap}: Each colored square shows whether Mistral-7B in-domain (few examples and evaluation examples come from the dataset in the row) has OOD performance (few examples from the row and evaluation from the column) that is at most 3\% lower than in-domain. If yes, we use fuller color, and we deem that train-test split questionable for studying OOD. We mark in-domain splits with X.}
  \label{fig:comment_splits}
\end{figure*}
